# Supplementary material for: RPT: Relational Pre-trained Transformer Is Almost All You Need towards Democratizing Data Preparation
Source: arXiv:2012.02469 source file (2021-03-31)
Supplement: Supplementary file 1 [file appendix.tex]

%!TEX root = paper.tex
\appendix

\section{Next Steps}

\subsection{\system-C: Data Cleaning}

Below is a list of (optional) research problems that we can selectively put in research papers.

\subsection*{Automatic Data Cleaning}

\stitle{Problem.}
Given a table $T$ with a set $\A$ of attributes, the problem of {\em automatic data cleaning} is to find a set of errors, denoted by $\error(T)$, where each element $e \in \error(T)$ is a cell $t[A]$ (a tuple and an attribute) of table $T$.
Each element $e$ is associated with a set of values, denoted by $\repair(e)$:
(i) $\repair(e) = \emptyset$ means that a repaired value is unknown;
(ii) $|\repair(e)| = 1$ indicates a unique repair; and 
(iii) $|\repair(e)| > 1$ means multiple possible repairs.

The above problem definition can generally cover all existing data cleaning solutions, and is easy to be extended to probabilistic solutions, where each error or a possible repair is associated with a probability.

As we have motivated earlier, existing solutions fall short of solving the data cleaning problem that the required ``signals'' or knowledge is outside of data $T$ at hand.
Hence, we will focus the data cleaning cases that are machine-hard but human-easy.

\stitle{Potential Issues.}
We can directly apply \system-C on $T$, masking the values tuple by tuple, attribute by attribute, or even token by token. 
If the value being masked and being predicted by \system-C don't match, we mark it as an error, and we can use the value from \system-C as the repair. 
This will work fine for certain columns, but clearly not all attributes, such as numeric attributes or those that are also ambiguous to humans.

The simplest way is that the user will specify which column to be scanned by \system-C, such as \at{name} or \at{gender}.
Alternatively, we may combine it with profiling tools to figure out which columns can be automatically cleaned?

\stitle{Demonstration.} 
You can imagine a demonstration scenario that a user uploads a table, and we can automatically flag errors and suggest repairs. Note that, this functionality is not surprising, but will be very interesting if we can show the cases that are machine-hard. 
Besides, it may be combined with some (collaborative) manual cleaning framework such as CoClean (\url{http://da.qcri.org/ntang/pubs/coclean.pdf}) for suggesting possible repairs.

\subsection*{Word-level Auto-completion}

\stitle{Problem.}
Consider a tuple $t$ with a set $\A$ of attributes, where $t[\A \setminus \{A\}]$ has full attribute values, but $t[A]$ has partial attribute values, denoted by $t[A] = \at{obs}$ (\ie the observed value).
The problem is to either predict \M$_p$ \at{obs} (the token that precedes \at{obs}), or \at{obs} \M$_s$ (the token that succeeds \at{obs}). Which direction to predict is decided by the user, by default the successor, because one is used to input a value from left to right, but sometimes it can also for the predecessor (\eg knowing someone's last name but not first name).

Note that, in the above definition, we assume that the value $t[A]$ is partial, but the tokens in \at{obs} are completed. For example, there is no first name like ``M''; instead, it should be ``Mike'' but the last name is missing.

\stitle{Potential Issues.}
We should provide top-$k$ predictions instead of top-1.

\subsection*{Character-level Auto-completion}

\stitle{Problem.} The problem is similar to the above word-level auto-completion, with the difference that:
(1) \at{obs} contains a partial token at the end of the observed value, \eg ``Mi''.
(2) we only want to auto-complete the last token (\eg ``Mi'' $\ra$ ``Mike''), instead of predicting the next token (\eg ``Jordan''). 

\stitle{Potential Issues.}
\system-C does not support this directly. If we mask the last partial token and ask \system-C to predict, it may not predict the token that do auto-completion.

Hence, we need a solution for character-level auto-completion.
(i) Training a character-level language model for this model might be too heavy, so intuitively it is not preferred. 
(ii) Instead, we might consider an algorithm to search the dictionary that start with the incomplete token, and then ask the trained model to select which one is the best fit.

\subsection*{Misspellings}

\stitle{Problem.}
Consider a tuple $t$ with a set $\A$ of attributes. The problem is to find which token in any attribute $t[A]$ is a misspelling, and correct it to its ground truth $t[A]^*$.

\stitle{Potential Issues.}
Similar to character-level auto-completion, if we mask a token and ask \system-C to predict it, we may get a token that is very different from the masked one. This cannot solve the misspelling problem. A typical assumption is that the misspelled token $x'$ and the real token $x$ are very similar, \ie with edit distance 1 or 2. Hence, we also need a search algorithm that can efficiently find possible tokens from the dictionary, and then use \system-C to select the most likely repair. 

In other words, we can consider it as ``repair with a constraint'' where the constraint is ``edit distance $\leq$ 2''. In practice, ``edit distance $=$ 1'' can cover 80\% of misspellings.

\subsection*{Miscellaneous: Domain Constraints}

Orthogonal to the above problems, we can consider domain constraints that can be defined or be automatically profiled. 
Such constraints may look like range $[20, 60]$. These constraints, if available, should be used to guide the solutions for various data cleaning problems.

\subsection{\system-E: Entity Resolution}

\subsection*{Entity Consolidation}

\stitle{Problem.}
Given a set $\mathcal{C} = \{C_1, \ldots, C_n\}$ of clusters, the problem is to ``consolidate'' each cluster $C_i$ into a unique entity $g_i$, called a golden record.

\stitle{Few-shot Learning.} 
The basic assumption is that there exists a ``criteria'' to pick, but the criteria is not easy to specify. A practical setting is to provide several examples, that are easy for human to understand. The question is, how \system-E can learn from these few examples. 

A cool idea called Pattern-Exploiting Training (PET) is introduced in~\cite{DBLP:journals/corr/abs-2001-07676}, which might be used for our problem. For example, if the examples are (iPhone 9, iPhone 10) $\ra$ iPhone 10 (\ie iPhone 10 is more preferred than iPhone 9), and (iPhone 10, iPhone 12) $\ra$ iPhone 12 (\ie iPhone 12 is more preferred than iPhone 10). We can use it to make the task clearly by asking questions iPhone 10 is \M~than iPhone 9 and iPhone 12 is \M~than iPhone 10, and enforce a language model to fill the two masks with the same value, \eg ``newer'' -- this is a discovered pattern from two examples, and this can better help the model to predict future golden records.
